# Supplementary material for: Emergence of a giant rotating cluster of fish in three dimensions by local interactions
Source: arXiv:2106.05892 ancillary file (2022-06-01)
Supplement: Supplementary file 1 [file JPSJ_arXiv_SUPPLEMENT.pdf]

# Supplemental Material for “Emergence of a Giant Rotating Cluster of Fish in Three Dimensions by Local Interactions”

Susumu Ito, and Nariya Uchida\*  
*Department of Physics, Tohoku University, Sendai, 980-8578, Japan*  
(Dated: May 24, 2022)

## CONTENTS

|                                                                               |    |
|-------------------------------------------------------------------------------|----|
| I. Comparison with Previous Studies                                           | 2  |
| II. Model and Parameters                                                      | 4  |
| III. Initial Conditions                                                       | 5  |
| IV. Classification of the Patterns and Measured Quantities                    | 6  |
| A. <i>Measured quantities</i>                                                 | 6  |
| B. <i>Classification of the patterns</i>                                      | 8  |
| C. <i>Ring and splitting</i>                                                  | 9  |
| D. <i>The principal moments of inertia of a solid torus</i>                   | 10 |
| V. Analysis of the Orbital Motion                                             | 11 |
| A. <i>Shift of the radial distance by the motion of the vortex axis</i>       | 11 |
| VI. The Size of a Rotating Cluster and Orbital Period                         | 13 |
| VII. Spatial Distribution                                                     | 16 |
| VIII. Qualitative Explanation for the Shape and the Mechanism of the Patterns | 17 |
| References                                                                    | 19 |

---

\* uchida@cmpt.phys.tohoku.ac.jp

## I. Comparison with Previous Studies

Most of the previous models for rotating clusters are two-dimensional [1, 2, 5–7, 9, 10, 12, 13]. Three dimensional models [3, 4, 8, 11] used hundreds of agents, which is an order of magnitude smaller than experimentally observed fish schools [17]. Few studies focus on the size of the cluster, and its dependence on the number of agents has not been investigated in detail. Below, we will examine the previous model studies [1–13] one by one. See also Table S1 which summarizes the type and results of previous models.

Refs. [1–4] use isotropic potentials with attraction and repulsion. In Ref. [1], additivity of attraction tends to make a rotating cluster in two dimensions (“mill”) smaller as the number of agents is increased. In a parameter region (called “region VI”), the interparticle distance tends to a finite minimum value as the number of agents increases, where the cluster exhibits rigid body rotation. Many patterns in common with Ref. [1] are also obtained in models with other types of potential (see Ref. [2] and the movie in it.). In Ref. [2], there is no parameter region which causes a finite minimum of the potential energy per agent in contrast to Ref. [1]. A phase diagram with patterns qualitatively similar to Ref. [1] is also obtained in Ref. [3], which uses the same potential as Ref. [1] but in three dimensions. A school (called “ball”) and a shell-shaped swarm (“shell”) mainly emerge, and rotating clusters are obtained in a narrower region than in Ref. [1]. Ref. [3] indicates that the size of a rotating cluster is smaller than the characteristic scale of interaction [15]. Ref. [4] introduced hydrodynamical long-range interactions into the model of Ref. [3], and showed that the patterns depend on the viscosity of fluid and pusher- or puller-type of the agents. The patterns in these models [1–4] depend on the initial conditions, and in particular, a school or a rotating cluster emerges for the same parameters.

Refs. [5–11] use asymmetrical interactions via a blind angle. Ref. [5] is an early study that introduced the blind angle, but it contains global attraction toward the center of mass of all agents, and thus individual agents use the information of the entire cluster. The model in Ref. [6] introduces attraction to the center of mass of neighboring agents in addition to the blind angle. Ref. [6] states that, in the non-blind angle case, the diameter of the cluster is less than the interaction range. In the blind angle case, the radius of the mill is less than the interaction range. As for the patterns, dynamically moving chain-like clusters appear by the effect of blind angle, in addition to the mill. These patterns also emerge in other models with similar interactions (see Ref. [7] and the movies in its supplemental material.). Ref. [8] extends the model of Ref. [6] to three dimensions and incorporates repulsion and global attraction. Without repulsion, a torus and a dynamical chain appear as in the two dimensional model. With repulsion, the agents do not aggregate if the global attraction is weak.

Ref. [9] incorporates a blind angle and a turning rate (maximal angular velocity in one time step) into the Vicsek model [18]. The turning rate is often used in discrete time-evolution models [9–11] to smoothen the angle of rotation in one time step as in continuous time-evolution models. Ref. [9] reports that the radius of the mill is always on the order of the interaction range. This statement on the cluster size holds even if the individual velocity is heterogeneous [10]. Ref. [11] is a three-dimensional model with zones of repulsion, attraction, and orientation. The cluster size is not shown in Ref. [11], which uses a hundred of agents.

Refs. [12, 13] introduce metric-free models using Voronoi tessellation in two dimensions, which are extensions of the model in Ref. [19]. Ref. [19] uses an asymmetrical interaction which includes a time evolution equation of angular velocity, but obtained no rotating clusters. Ref. [12] introduced a blind angle factor into the model of Ref. [19], and obtained a milling cluster. Ref. [13] further adds hydrodynamic interaction to the model of Ref. [12], and finds a rotating cluster that is much larger than the swimmer size. In both Ref. [12] and Ref. [13], the rotational order parameter is peaked at several hundreds of agents, and then decreases as the number of agents is increased.

From what are stated above, we may say that there is no previous study that investigates a rotating cluster with several thousands of agents in three dimensions. We showed a new model for the emergence of a giant rotating cluster.

TABLE S1. List of the previous models related to this paper. The name of the patterns are basically those used in the previous studies, but some names are changed for unification. For example, “flock” and “liquid” are reworded as “school”. The interaction range and the cluster size are those for which rotating clusters appear. “ACM” is an abbreviation for “attraction to the center of mass of neighboring particles”.

| reference                          | dimension | interaction type                                                                     | number of agents                                  | principal patterns                                                     | interaction range                                                       | the rotating cluster size                                                                                                                         |
|------------------------------------|-----------|--------------------------------------------------------------------------------------|---------------------------------------------------|------------------------------------------------------------------------|-------------------------------------------------------------------------|---------------------------------------------------------------------------------------------------------------------------------------------------|
| D’Orsogna <i>et al.</i> (2006) [1] | two       | Morse potential                                                                      | 40 ~ 600                                          | gas, school, and mills (disk, annulus, ring)                           | attenuation length of the attraction $l_a = 1 \sim 2$                   | A cluster is generally smaller as the number of agents is increased.                                                                              |
| Cheng <i>et al.</i> (2016) [2]     | two       | extention of potential as used in Ref. [14]                                          | 30 ~ 400                                          | gas, crystal, school, mills (disk, annulus, ring), and undirected mill | The length at which the potential is cut off $\alpha d = 0.75 \sim 1.5$ | A rotating cluster is smaller as the number of agents is increased.                                                                               |
| Nguyen <i>et al.</i> (2012) [3]    | three     | Morse potential                                                                      | 600                                               | gas, school, torus, and ring                                           | attenuation length of the attraction $l_a \gtrsim 1$                    | on the order of 0.01 ~ 0.1 [15]                                                                                                                   |
| Chuang <i>et al.</i> (2016) [4]    | three     | Morse potential, and hydrodynamic interaction                                        | 50 ~ 250                                          | gas, school, and torus                                                 | hydrodynamical long-range interaction                                   | not shown                                                                                                                                         |
| Shimoyama <i>et al.</i> (1996) [5] | two       | potential as used in Ref. [14], blind angle factor, and globally attraction          | 10 ~ 50                                           | swarm, school, and mill                                                | global attraction                                                       | not shown                                                                                                                                         |
| Strömbom (2011) [6]                | two       | ACM, and blind angle                                                                 | 50 ~ 100                                          | swarm, school, mill, undirected mill, and chain                        | radius of interaction $R = 4$                                           | In the non-blind angle case, the diameter of the cluster is less than $R$ . In the blind angle case, the radius of the cluster is less than $R$ . |
| Barberis <i>et al.</i> (2016) [7]  | two       | ACM, and blind angle                                                                 | 10000 (They split into dozens of small clusters.) | gas, swarm, string, undirected mill, and chain                         | radius of interaction $R_0 = 1$                                         | not shown                                                                                                                                         |
| Strömbom <i>et al.</i> (2015) [8]  | three     | ACM, blind angle, repulsion, and globally attraction                                 | 50 ~ 100                                          | string, school, torus, and chain                                       | global attraction                                                       | not shown                                                                                                                                         |
| Costanzo <i>et al.</i> (2018) [9]  | two       | orientational interaction, blind angle, and turning angle                            | 1000                                              | string, school, and mill                                               | radius of interaction $r = 1$                                           | The radius of the cluster is on the order of $r$ .                                                                                                |
| Costanzo (2019) [10]               | two       | orientational interaction, blind angle, and turning angle                            | 1000                                              | school and mill                                                        | radius of interaction $r = 1$                                           | The radius of the cluster is on the order of $r$ .                                                                                                |
| Couzin <i>et al.</i> (2002) [11]   | three     | attractive, repulsive, and orientational interaction, blind angle, and turning angle | 10 ~ 100                                          | swarm, school, and torus                                               | the radius of attraction $r_a \gtrsim 14$ ( $\Delta r_a \gtrsim 10$ )   | not shown                                                                                                                                         |
| Calovi <i>et al.</i> (2014) [12]   | two       | anisotropic potential, and blind angle                                               | 10 ~ 4000                                         | string, school, and mill                                               | Voronoi tessellation                                                    | not shown                                                                                                                                         |
| Filella <i>et al.</i> (2018) [13]  | two       | anisotropic potential, blind angle, and hydrodynamical long-range interaction        | 10 ~ 1000                                         | swarm, school, and mill                                                | Voronoi tessellation, and hydrodynamical long-range interaction         | the cluster size is much larger than the swimmer size [16].                                                                                       |

## II. Model and Parameters

First, we illustrate the interaction capacity and dynamic control of the attraction strength in the model. Fig. S1(a)-(c) schematically shows the example of  $\mathcal{L}_i$ ,  $\mathcal{A}_i$ , and  $\Lambda_i$  for  $N_u = 3$ . In Fig. S1(c), the positions of the other agents around the  $i$ -th agent at  $t = t^*, t^{**}$  corresponds to the situation shown in Fig. S1(a). This is the case where the agent is out of a cluster, and is attracted by every other agent in the radius  $r_a$ . At  $t = t^* + \tau$ , the positions of the agents correspond to those shown in Fig. S1(b). This means that the agent is back in a cluster and only the orientational and repulsive interactions with the  $N_u$  neighbors remain. At  $t = t^{**} + \tau$ , the situation shown in Fig. S1(a) still continues, and then the attraction is maintained for another period  $\tau$ .

Next, we explain the correspondence between the parameters used in this model and the experiments. The sustained speed  $v_0$  is the swimming speed that can last almost indefinitely, and its value is approximately  $0.5 \sim 5 \text{ BL s}^{-1}$ . Many fish, however, have  $1 \sim 3 \text{ BL s}^{-1}$  for  $v_0$  [22–27]. In the numerical simulation, time is rescaled by the characteristic time  $\tau_0$ . It is reasonable to define  $\tau_0$  from the relation between the typical velocity  $v_0$  and acceleration of fish. The acceleration is on the order of  $0.1 \sim 1 \text{ BL s}^{-2}$  both when the fish is perturbed by flow [26, 27], and when it is interacting with other fish in the radius  $r_e$  [21]. We thus adopt  $\tau_0 = 1 \text{ sec}$  as the time constant. Moreover, The value of the maximum speed of fast-start ranges between  $5.3 \text{ BL s}^{-1}$  and  $27.3 \text{ BL s}^{-1}$ , but many fish have  $7 \sim 11 \text{ BL s}^{-1}$  [23, 28]. The value of  $v_a$  is adopted from this range. Table S2 summarizes the set of parameters.

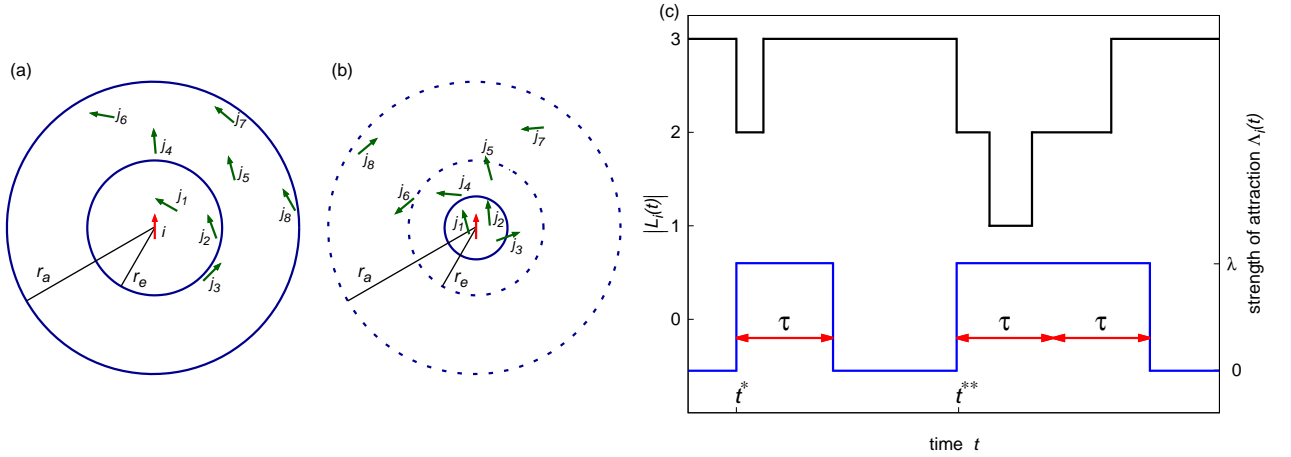

FIG. S1. Schematic illustration of (a)-(b) the range of interactions and (c) the duration of fast-start for  $N_u = 3$ . In (a) and (b), the  $i$ -th agent in the center (red arrow) is surrounded by the neighbors  $j_1 \sim j_8$  (green arrows) that are numbered by the proximity to  $i$ . The blue circles show the radii of interactions (solid: effective, dashed: nominal). (a) The  $i$ -th agent has orientational and repulsive interactions with  $j_1$  and  $j_2$ , and attraction with  $j_3 \sim j_8$ :  $\mathcal{L}_i = \{j_1, j_2\}$  and  $|\mathcal{L}_i| = 2$ ;  $\mathcal{A}_i = \{j_3, j_4, j_5, j_6, j_7, j_8\}$  and  $|\mathcal{A}_i| = 6$ . (b) The  $i$ -th agent has the orientational and repulsive interactions with the three neighbors  $j_1, j_2$ , and  $j_3$  ( $\mathcal{L}_i = \{j_1, j_2, j_3\}$  and  $|\mathcal{L}_i| = 3$ ), and the attraction is turned off. The effective radius of interaction is thus equal to the distance to  $j_3$ . (c) Time evolution of the number of agents in the interaction range  $|\mathcal{L}_i(t)|$  (black) and the strength of attraction  $\Lambda_i(t)$  (blue). Attraction is turned on at the moments when  $|\mathcal{L}_i(t)|$  becomes less than three ( $t = t^*, t^{**}$ ), and lasts for a period  $\tau$ . At  $t = t^* + \tau$ , the attraction is turned off because  $|\mathcal{L}_i(t)| = 3$ . At  $t = t^{**} + \tau$ , we have  $|\mathcal{L}_i(t)| < 3$  and the attraction is maintained for another period until we get  $|\mathcal{L}_i(t)| = 3$  at  $t = t^{**} + 2\tau$ .

TABLE S2. List of parameters employed in the model. This model uses the rescaled units of length and time ( $r_e = 1.5$  BL  $= 1$ ,  $\tau_0 = 1$  s  $= 1$ ).

| symbol    | definition                   | experimental value                    | adopted value           | rescaled value  |
|-----------|------------------------------|---------------------------------------|-------------------------|-----------------|
| $r_e$     | radius of equilibrium        | $\sim 1.5$ BL [20, 21]                | 1.5 BL                  | 1               |
| $r_a$     | radius of attraction         | $\gtrsim 5$ BL [20, 21]               | 7.5 BL                  | 5               |
| $r_b$     | body length                  | 1 BL                                  | 1 BL                    | 2/3             |
| $v_0$     | sustained speed              | $0.5 \sim 5$ BL s $^{-1}$ [22–27]     | $1.5$ BL s $^{-1}$      | 1               |
| $v_r$     | speed of collision avoidance | –                                     | $1.5$ BL s $^{-1}$      | 1               |
| $\tau_0$  | characteristic time-scale    | $\sim 1$ s [21–27]                    | 1 s                     | 1               |
| $v_a$     | speed of fast-start          | $5.3 \sim 27.3$ BL s $^{-1}$ [23, 28] | $7.5$ BL s $^{-1}$      | 5               |
| $\tau$    | duration of fast-start       | $0.03 \sim 0.18$ s [28, 29]           | 0.10 s                  | 0.10            |
| $N_u$     | interaction capacity         | –                                     | computational parameter | $1 \sim 50$     |
| $\lambda$ | strength of attraction       | –                                     | computational parameter | $0.2 \sim 25.0$ |

### III. Initial Conditions

Depending on the box size  $L$ , we use two kinds of initial conditions: (i) For  $L = 35$  or  $40$ , the agents have randomly distributed positions and directions, and have the same speed  $v_0$  at  $t = 0$ ; (ii) for  $L = 120$ , a single spherical cluster

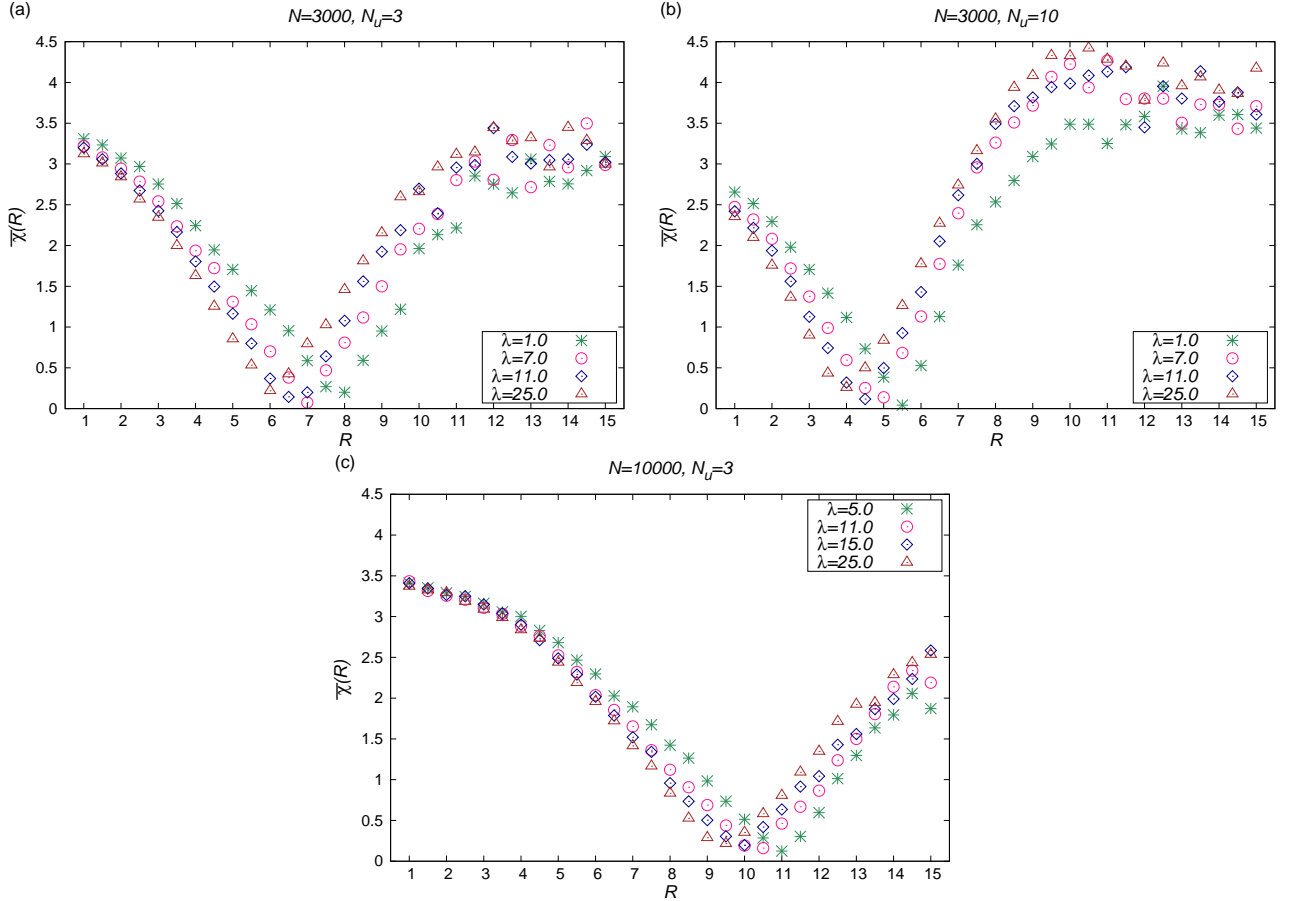

FIG. S2. Examples of determination of  $R_\chi$ . (a)  $N = 3000, N_u = 3, \lambda = 1.0$  (star),  $\lambda = 7.0$  (circle),  $\lambda = 11.0$  (diamond),  $\lambda = 25.0$  (triangle). For example, the function  $\bar{\chi}(R)$  is minimized at  $R_\chi = 8.0$  when  $\lambda = 1.0$ . (b)  $N = 3000, N_u = 10, \lambda = 1.0$  (star),  $\lambda = 7.0$  (circle),  $\lambda = 11.0$  (diamond),  $\lambda = 25.0$  (triangle). (c)  $N = 10000, N_u = 3, \lambda = 5.0$  (star),  $\lambda = 11.0$  (circle),  $\lambda = 15.0$  (diamond),  $\lambda = 25.0$  (triangle).

in which the agents contact each other with the distance almost equal to  $r_e$  at  $t = 0$ . The purpose of using the initial condition (i) is to show that rotating clusters spontaneously emerge from a random state. The values of the box sizes  $L = 35, 40$  are chosen appropriately to reduce computational costs. If  $L$  is too large, the agents form several clusters from the random distribution and it will take a very long time for them to collide with each other and form one cluster. A too small  $L$ , however, brings about finite size effects. The initial condition (ii) has two advantages. First, we can examine the stability of a one-cluster state: If one cluster is unstable, it will split into several clusters. Second, depending on the parameters, a giant rotating cluster with a large hole in the center (“ring”) emerges, which causes finite-size effects due to the periodic boundary condition for small  $L$ . Using the initial condition (ii),  $L$  can be taken large enough, thus we set  $L = 120$  which does not cause a finite size effect.

For the initial condition (ii), the radius of the initial cluster is determined as follows. At  $t = 0$ , the agents are randomly distributed in a sphere of radius  $R$  and have the same direction ( $\mathbf{v}_i(t=0) = (v_0, 0, 0)$ ). If  $R$  is too small, the cluster will split by repulsive interaction. On the other hand, if  $R$  is too large, the agents will split into many clusters by attraction, and it takes long time for them to reunite and form one cluster. Therefore, we need to choose an optimal radius  $R_\chi$  for which the cluster keeps the initial radius  $R$  over a short period of time. To find the optimal radius  $R_\chi$  for each parameter set  $(N, N_u, \lambda)$ , we define the deviation from a sphere with the initial radius  $R$  as

$$\chi(R, t) = \left| \frac{S_1(t) + S_2(t) + S_3(t)}{3} - R \right|, \quad (\text{S1})$$

where  $R$  ranges from 1 to 15 with the increment 0.5,  $S_1(t), S_2(t), S_3(t)$  are the cluster sizes in the direction of eigenvectors of the moments of inertia tensor, and the time step  $dt = 0.001$  is used (See Eq. S9 for the definition of  $S_1, S_2$ , and  $S_3$ ). Then we define  $R_\chi$  for the initial condition as the radius that minimizes the time-averaged  $\chi(R, t)$  between  $t = 0$  and  $t = 10$  (which is denoted by  $\bar{\chi}(R)$ ). See Fig. S2 for specific examples of  $\bar{\chi}(R)$ . Here we use the aligned initial conditions, which is important for testing the stability of a cluster. If we use a randomly oriented initial configuration and the cluster splits, we cannot distinguish whether the splitting is due to the orientational interaction or the repulsive interaction.

#### IV. Classification of the Patterns and Measured Quantities

##### A. Measured quantities

We perform the cluster judgement as follows: an agent belongs to a cluster if its distance from the nearest agent is smaller than  $r_a$ . Let  $\mathcal{C}$  be a set of agents that belong to the largest cluster. The cluster percentage

$$p_c(t) = |\mathcal{C}(t)|/N \quad (\text{S2})$$

represents the ratio of the number of agents in the largest cluster to the total number of agents, and is used to investigate the instability of the cluster. The polar order parameter

$$\mathbf{P}(t) = \frac{1}{|\mathcal{C}|} \sum_{i \in \mathcal{C}} \frac{\mathbf{v}_i(t)}{|\mathbf{v}_i(t)|} \quad (\text{S3})$$

and the rotational order parameter

$$\mathbf{M}(t) = \frac{1}{|\mathcal{C}|} \sum_{i \in \mathcal{C}} \frac{\mathbf{c}_i(t) \times \mathbf{v}_i(t)}{|\mathbf{c}_i(t)| |\mathbf{v}_i(t)|} \quad (\text{S4})$$

are the essential quantities that distinguish between polarized school and rotating clusters, where  $\mathbf{c}_i = \mathbf{r}_i - \mathbf{r}_G$  with  $\mathbf{r}_G$  being the center of mass position of the cluster, and  $\times$  the cross product operator. We define the radial position  $\mathbf{c}_i^\perp$  as the projection of  $\mathbf{c}_i$  onto a vector which is perpendicular to  $\mathbf{M}(t)$  and  $\mathbf{c}_i \times \mathbf{M}(t)$ . The outer and inner radii of the maximum cluster are defined as

$$R_o(t) = \max_{i \in \mathcal{C}} |\mathbf{c}_i^\perp(t)|, \quad (\text{S5})$$

and

$$R_i(t) = \min_{i \in \mathcal{C}} |\mathbf{c}_i^\perp(t)|, \quad (\text{S6})$$

respectively. The rotation period at each time is obtained from the agent-averaged angular velocity

$$\Omega(t) = \frac{1}{|\mathcal{C}|} \left| \sum_{i \in \mathcal{C}} \frac{\mathbf{c}_i^\perp(t) \times \mathbf{v}_i(t)}{|\mathbf{c}_i^\perp(t)|^2} \right|. \quad (\text{S7})$$

The moments of inertia tensor

$$I_{\mu\nu}(t) = \sum_{i \in \mathcal{C}} (\mathbf{c}_i^2(t) \delta_{\mu\nu} - c_{i,\mu}(t) c_{i,\nu}(t)) \quad (\text{S8})$$

helps to characterize the shape of the cluster, where  $\mu, \nu = x, y, z$  and  $\delta_{\mu\nu}$  is the  $\mu, \nu$ -component of the identity matrix. We obtain the principal moments of inertia  $I_1(t), I_2(t), I_3(t)$  ( $I_1(t) \geq I_2(t) \geq I_3(t)$ ) and normalized eigenvectors  $\mathbf{u}_1(t), \mathbf{u}_2(t), \mathbf{u}_3(t)$  by diagonalizing this tensor. The cluster sizes  $S_1(t), S_2(t), S_3(t)$  in the direction of eigenvectors are defined by

$$S_\alpha(t) = \max_{i \in \mathcal{C}} |\mathbf{c}_i(t) \cdot \mathbf{u}_\alpha(t)|, \quad (\text{S9})$$

where  $\alpha = 1, 2, 3$ . The ratio of principal moments of inertia

$$I_s(t) = \frac{I_1(t)}{(I_2(t) + I_3(t))/2} \quad (\text{S10})$$

is defined as the ratio regarding the shape of the torus. If the shape of the cluster is a solid torus with the inner radius  $R_i$  and outer radius  $R_o$ , the ratio becomes

$$I_s = \frac{8(R_o + R_i)^2 + 6(R_o - R_i)^2}{4(R_o + R_i)^2 + 5(R_o - R_i)^2} \quad (\text{S11})$$

as we show below (see Eq. S17). This ratio equals to 2 when  $R_i = R_o$ , and

$$I_s = \frac{14}{9} \quad (\text{S12})$$

for  $R_i = 0$ .

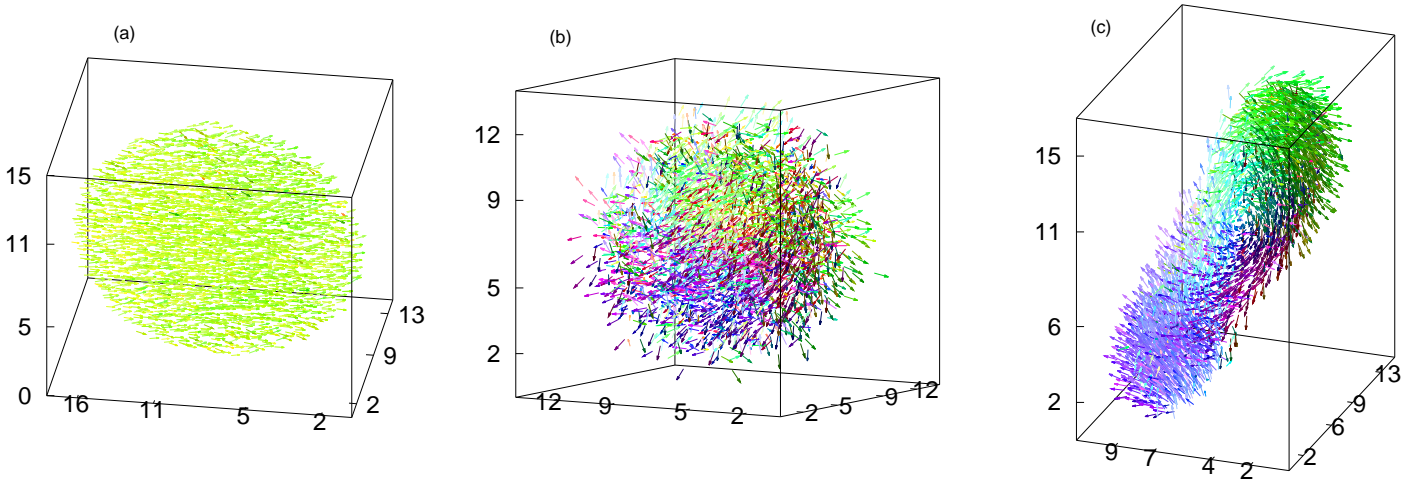

FIG. S3. Snapshots of non-rotating fish clusters. Agents are represented in the same way as in Fig. 1. (a) A polarized school for  $N = 3000, N_u = 3, \lambda = 0.5$ . (b) A swarm for  $N = 3000, N_u = 1, \lambda = 25.0$ . (c) Undetermined form for  $N = 3000, N_u = 10, \lambda = 9.0$ .

### B. Classification of the patterns

We classify the clusters into 7 patterns: (i) rotating ball, (ii) torus, (iii) ring, (iv) polarized school (see Fig. S3(a) and Movie S6 in Ref. [30]), (v) swarm (see Fig. S3(b)), (vi) splitting (see Movie S8 in Ref. [30]), and (vii) undetermined form (see Fig. S3(c)). As shown in Fig. S4,  $P(t)$ ,  $M(t)$ ,  $R_o(t)$ , and  $R_i(t)$  converge in a few hundred computational time units if the cluster is stable.

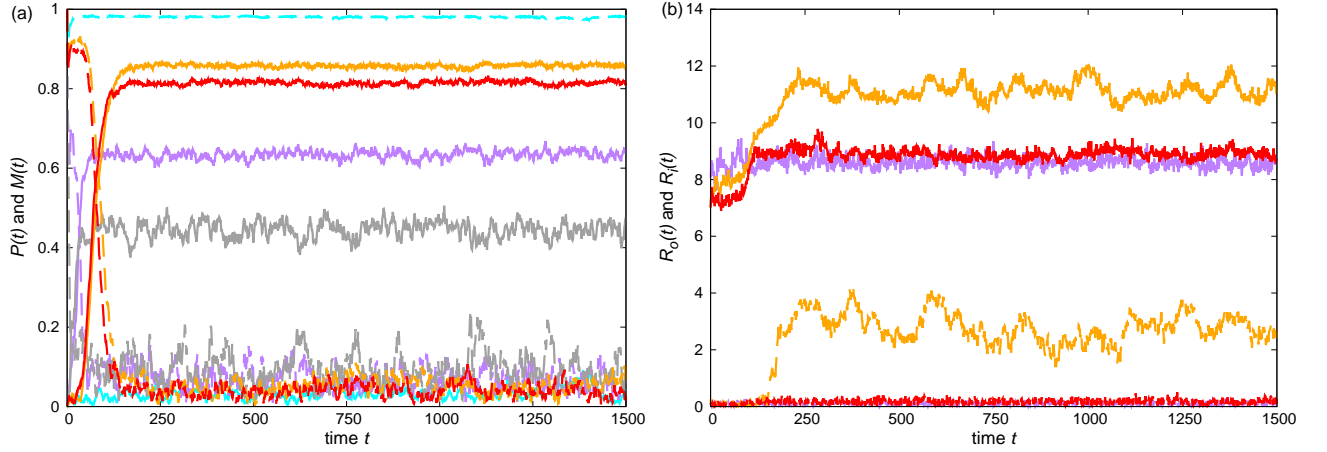

FIG. S4. Time evolution of the order parameters and cluster radii with the initial condition (ii) and  $N = 3000$ . Each line corresponds to the parameters as follows. Cyan:  $N_u = 3$  and  $\lambda = 0.5$  (polarized school). Grey:  $N_u = 1$  and  $\lambda = 25.0$  (swarm). Orange:  $N_u = 3$  and  $\lambda = 5.0$  (ring). Red:  $N_u = 3$  and  $\lambda = 9.0$  (torus). Purple:  $N_u = 1$  and  $\lambda = 7.0$  (rotating ball). (a)  $P(t)$  is shown by the solid line, and  $M(t)$  the dashed line. (b) The solid line and dashed lines represent  $R_o(t)$  and  $R_i(t)$ , respectively. These quantities reach steady values in a few hundred computational time units and converge sufficiently by  $t = 1000$  when we start time-averaging.

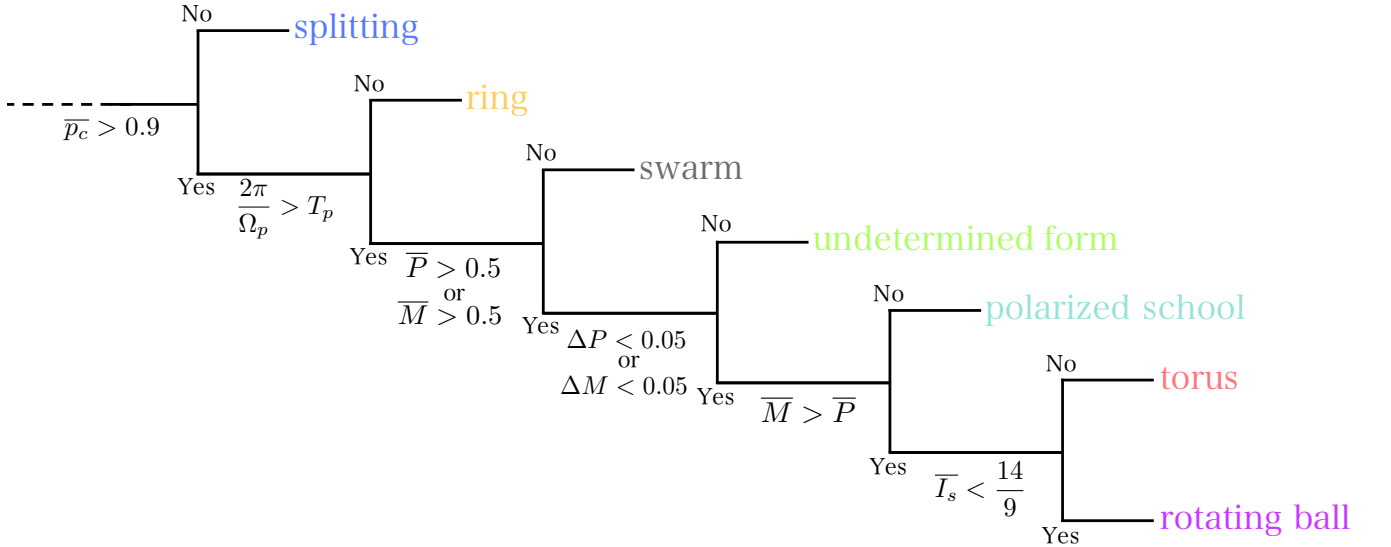

FIG. S5. Dendrogram of classification. Each cluster is screened by the conditions listed from the left to right.

We define  $\bar{X}$  as the time-average of any quantity  $X(t)$  over the interval  $[t - 500, t]$ . The standard deviations of  $P(t)$  and  $M(t)$  over the same interval are denoted as  $\Delta P$  and  $\Delta M$ , respectively. We identified the periods in which  $R_i(t) \geq r_e$ , and defined  $T_p$  as the maximum duration of those periods in a single simulation, and  $\Omega_p$  as the average of  $\Omega(t)$  over those periods. The actual classification of patterns is performed according to Fig. S5. The first condition is about whether one cluster can be maintained. The second condition tells whether the duration  $T_p$  is longer than the average time  $2\pi/\Omega_p$  that it takes for each agent to circle the cluster. The third condition is about the polar

orientational order and rotational order. Fluctuation of the cluster shape is determined by the fourth condition, in which the threshold value 0.05 is chosen because  $\Delta P$  and/or  $\Delta M$  are in the range  $0.001 \sim 0.01$  for polarized schools, tori, and rotating balls. The fifth condition judges the rotational order of the cluster, and the sixth condition is about the shape of a rotating cluster. The value  $14/9$  is based on Eq. S12.

### C. Ring and splitting

Note that it takes a long time for a ring and a cluster of undetermined form to split. In particular, a ring sometimes tears off and splits. This process is understood as follows. First, the ring is torn off by fluctuations of number density of agents, and takes a worm-like shape. The worm-like cluster has further density fluctuations and sometimes splits (see Movie S8 in Ref. [30]). In the case where splitting doesn't occur, the worm-like cluster starts to rotate from its front and forms a ring again (see Movie S7 in Ref. [30]). With appropriate parameter values ( $\lambda, N_u$ ), this time interval is more than 100 times as large as the time-averaged orbital period  $\bar{T}_b$  (see Fig. S6, Eq. S25, and Fig. S11(b)). The ring, therefore, can maintain its state for a long time compared to the characteristic time-scale of each agent, in spite of the fact that it has a large hole. In connection with this, the classification between splitting and ring (or splitting and undetermined form) in the phase diagram using data in the interval  $t < 1500$  is a rough one. It is difficult to determine the appropriate simulation time for the classification between splitting and ring, because it includes two indefinite factors: there is the indefiniteness of the time interval at which tearing-off occurs as shown in Fig. S6, and tearing-off doesn't necessarily leads to splitting as shown in Fig. S7(b).

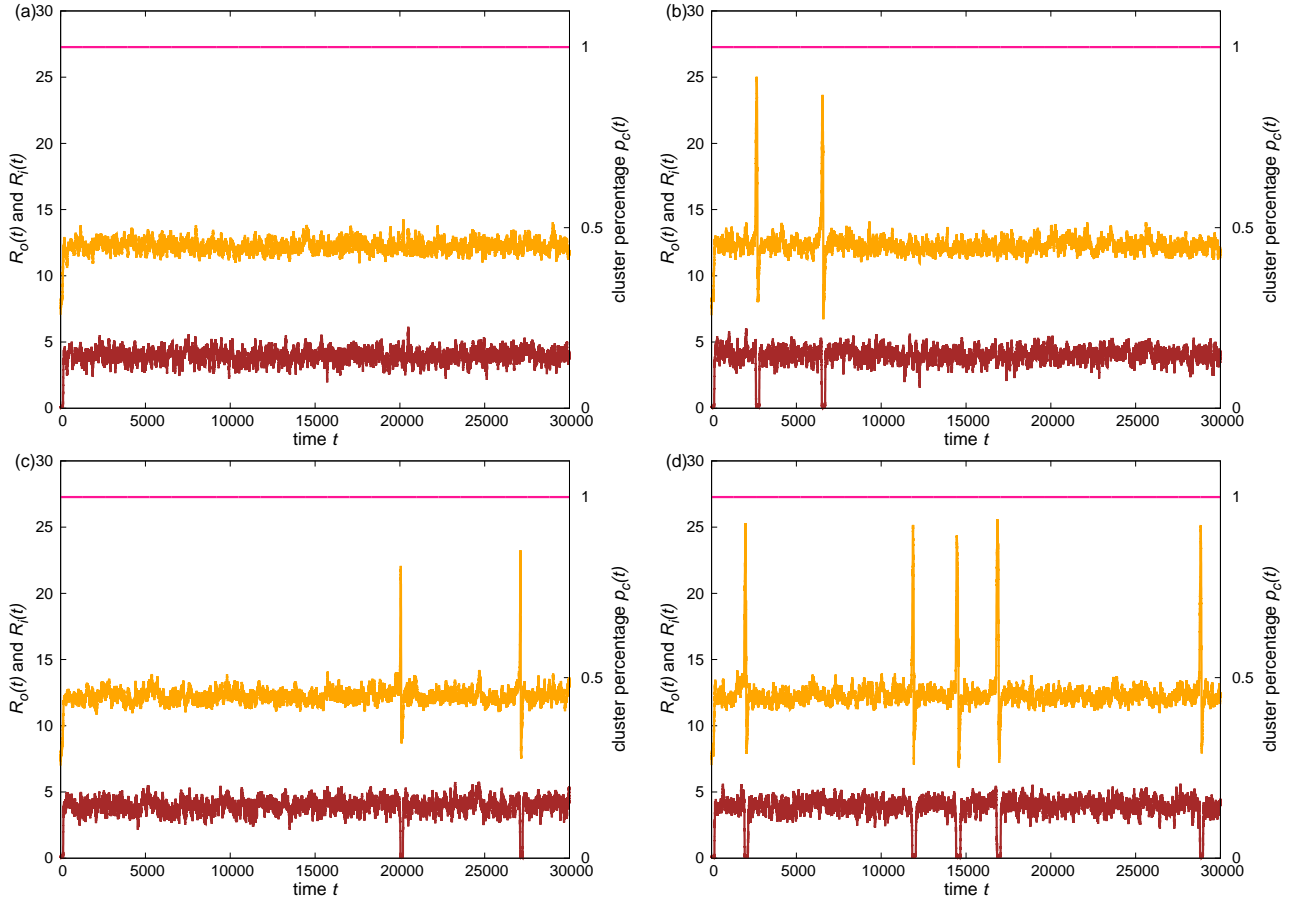

FIG. S6. Time interval between tearing-off for  $N = 3000, N_u = 3$ , and  $\lambda = 4.0$  with the initial condition (ii). The orange, brown, and magenta lines are  $R_o(t)$ ,  $R_l(t)$ , and  $p_c(t)$ , respectively. No splitting occurs in all cases from (a) to (d). (a) A case where tearing-off never occurs in the simulation time  $0 < t < 30000$ . (b)-(d) Tearing-off is observed at different time with various time intervals.

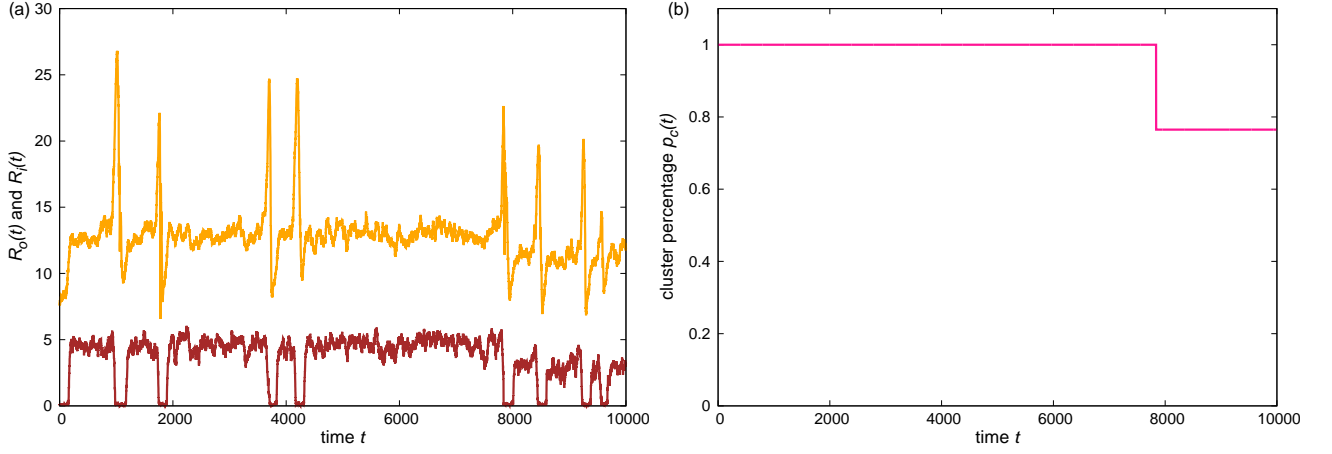

FIG. S7. Example of tearing-off and splitting of a ring with  $N = 3000$ ,  $N_u = 3$ , and  $\lambda = 3.5$ . We use the initial condition (ii). In (a), tearing-off and recovery repeat 4 times in the ring having  $R_i(t) \approx 5$  (brown line) by  $t = 5000$ . When it is torn off, the cluster becomes worm-shaped, then  $R_o(t)$  (orange line) has a spike and  $R_i(t)$  falls to zero (see also Movie S7 in Ref. [30]). After this, a splitting occurs at  $t \sim 8000$  by tearing-off of the worm-shaped cluster (see Movie S8 in Ref. [30]), and more than 20% of the agents are lost from the largest cluster (see (b) in this figure). It begins to tear off and recover again, after splitting.

#### D. The principal moments of inertia of a solid torus

Let us derive the principal moments of inertia of a solid torus with the inner radius  $R_i$ , outer radius  $R_o$  and mass  $m$ . We define the constants  $a = (R_o + R_i)/2$  (major radius) and  $b = (R_o - R_i)/2$  (minor radius), and the parameters  $\rho \in [0, b]$  and  $\phi, \psi \in [0, 2\pi)$ . A position inside the torus is expressed in Cartesian coordinates as follows.

$$\begin{cases} x = (a + \rho \cos \psi) \cos \phi, \\ y = (a + \rho \cos \psi) \sin \phi, \\ z = \rho \sin \psi. \end{cases} \quad (\text{S13})$$

The volume, density, and Jacobian are  $V = 2\pi^2 ab^2$ ,  $\sigma = m/V$ , and

$$\begin{aligned} J &= \begin{vmatrix} \frac{\partial x}{\partial \rho} & \frac{\partial x}{\partial \phi} & \frac{\partial x}{\partial \psi} \\ \frac{\partial y}{\partial \rho} & \frac{\partial y}{\partial \phi} & \frac{\partial y}{\partial \psi} \\ \frac{\partial z}{\partial \rho} & \frac{\partial z}{\partial \phi} & \frac{\partial z}{\partial \psi} \end{vmatrix} \\ &= \begin{vmatrix} \cos \psi \cos \phi & -(a + \rho \cos \psi) \sin \phi & -\rho \sin \psi \cos \phi \\ \cos \psi \sin \phi & (a + \rho \cos \psi) \cos \phi & -\rho \sin \psi \sin \phi \\ \sin \psi & 0 & \rho \cos \psi \end{vmatrix} \\ &= \rho(a + \rho \cos \psi), \end{aligned} \quad (\text{S14})$$

respectively. Firstly, we calculate the principal moment of inertia  $I_1$  about the axis passing through the center and perpendicular to the diameter:

$$\begin{aligned} I_1 &= \sigma \int_{\text{torus}} dV (x^2 + y^2) \\ &= \sigma \int_0^b d\rho \int_0^{2\pi} d\phi \int_0^{2\pi} d\psi \rho (a + \rho \cos \psi) (a + \rho \cos \psi)^2 \\ &= 2\pi\sigma \int_0^b d\rho \int_0^{2\pi} d\psi (a^3 \rho + 3a\rho^3 \cos^2 \psi) \\ &= 2\pi^2 ab^2 \sigma \left( a^2 + \frac{3b^2}{4} \right) \\ &= \frac{m}{8} (8a^2 + 6b^2). \end{aligned} \quad (\text{S15})$$

Note that the odd power of trigonometric function disappear by integration with respect to  $\psi$ . Secondly, the two principal moments of inertia  $I_2, I_3$  about the  $x$  and  $y$ -axis are equal because of the rotational symmetry about the  $z$ -axis. We calculate  $I_2$  as:

$$\begin{aligned}
I_2 &= \sigma \int_{torus} dV (y^2 + z^2) \\
&= \sigma \int_0^b d\rho \int_0^{2\pi} d\phi \int_0^{2\pi} d\psi \rho (a + \rho \cos \psi) \\
&\quad \times ((a + \rho \cos \psi) \sin \phi)^2 + (\rho \sin \psi)^2 \\
&= \pi \sigma \int_0^b d\rho \int_0^{2\pi} d\psi (a^3 \rho + a \rho^3 (2 + \cos^2 \psi)) \\
&= 2\pi^2 ab^2 \sigma \left( \frac{a^2}{2} + \frac{5b^2}{8} \right) \\
&= \frac{m}{8} (4a^2 + 5b^2).
\end{aligned} \tag{S16}$$

Obviously  $I_1$  is larger than  $I_2$  and  $I_3$ , and the ratio is

$$\frac{I_1}{I_2} = \frac{I_1}{I_3} = \frac{8a^2 + 6b^2}{4a^2 + 5b^2} = \frac{8(R_o + R_i)^2 + 6(R_o - R_i)^2}{4(R_o + R_i)^2 + 5(R_o - R_i)^2}. \tag{S17}$$

## V. Analysis of the Orbital Motion

We define  $\mathbf{e}_M(t) = \mathbf{M}(t)/M(t)$  as the unit vector along the vortex axis. Let  $\mathbf{e}_1^\perp(t)$  be the vector perpendicular to  $\mathbf{e}_M(t)$ :

$$\mathbf{e}_1^\perp(t) = (I - \mathbf{e}_M(t) \otimes \mathbf{e}_M(t)) \mathbf{e}_x, \tag{S18}$$

where  $I$  is the identity matrix, and  $\otimes$  is the tensor product operator and  $\mathbf{e}_x$  is the unit vector along the  $x$ -axis. The other axis perpendicular to  $\mathbf{e}_M(t)$  is defined by

$$\mathbf{e}_2^\perp(t) = \mathbf{e}_M(t) \times \mathbf{e}_1^\perp(t). \tag{S19}$$

Then the in-plane position

$$\mathbf{c}_i^\perp(t) = (c_{i,1}^\perp(t), c_{i,2}^\perp(t)) = (\mathbf{c}_i(t) \cdot \mathbf{e}_1^\perp(t), \mathbf{c}_i(t) \cdot \mathbf{e}_2^\perp(t)) \tag{S20}$$

describes the orbit of the  $i$ -th agent projected onto a plane perpendicular to the vortex axis. The azimuthal angle  $\phi \in [-\pi, \pi)$  is obtained as

$$\phi_i(t) = \tan^{-1} \left( \frac{c_{i,2}^\perp(t)}{c_{i,1}^\perp(t)} \right). \tag{S21}$$

Fig. S8 shows time-evolution of  $c^\perp, c_1^\perp$  for a torus.

We define the autocorrelation function of the radial distance  $c_i^\perp(t) = |\mathbf{c}_i(t)|$  by

$$G(\Delta t) = \frac{1}{|\mathcal{C}|} \sum_{i \in \mathcal{C}} \left( \langle c_i^\perp(t + \Delta t) c_i^\perp(t) \rangle - \langle c_i^\perp(t) \rangle^2 \right), \tag{S22}$$

where  $\langle \dots \rangle$  represents the time-average. This function is further normalized by requiring  $G(\Delta t = 0) = 1$  in Fig. S9(a).

### A. Shift of the radial distance by the motion of the vortex axis

Let us calculate the shift of the radial distance by the motion of the vortex axis. As shown in Fig. S9(b), the vortex axis  $\mathbf{e}_M(t)$  at  $t$  becomes  $\mathbf{e}_M(t + \delta t)$  after an infinitesimal time  $\delta t$ , with the angle shift  $\delta \theta_M$ . Assuming that the agent is not moving and is fixed at a certain point in the space, we calculate the relation between  $c^\perp(t)$  and

$c^\perp(t + \delta t)$ . The coordinates after an infinitesimal time  $\delta t$  is obtained by rotating the initial coordinate axes such that  $\mathbf{e}_M(t)$  (black solid arrow) is moved to  $\mathbf{e}_M(t + \delta t)$  (black dashed arrow) by the rotation angles  $\phi_M$  and then  $\delta\theta_M$  as shown in Fig. S9(b). The distances  $c^\perp(t)$  and  $c^\parallel(t)$  are transformed as follows.

$$\begin{aligned} & \begin{bmatrix} 1 & 0 & 0 \\ 0 & \cos \delta\theta_M & \sin \delta\theta_M \\ 0 & -\sin \delta\theta_M & \cos \delta\theta_M \end{bmatrix} \begin{bmatrix} \cos \phi_M & \sin \phi_M & 0 \\ -\sin \phi_M & \cos \phi_M & 0 \\ 0 & 0 & 1 \end{bmatrix} \begin{bmatrix} 0 \\ c^\perp(t) \\ c^\parallel(t) \end{bmatrix} \\ &= \begin{bmatrix} c^\perp(t) \sin \phi_M \\ c^\perp(t) \cos \delta\theta_M \cos \phi_M + c^\parallel(t) \sin \delta\theta_M \\ -c^\perp(t) \sin \delta\theta_M \cos \phi_M + c^\parallel(t) \cos \delta\theta_M \end{bmatrix}. \end{aligned} \quad (\text{S23})$$

Therefore, we get

$$\begin{aligned} c^\perp(t + \delta t) &= \left[ (c^\perp(t) \sin \phi_M)^2 + (c^\perp(t) \cos \delta\theta_M \cos \phi_M + c^\parallel(t) \sin \delta\theta_M)^2 \right]^{\frac{1}{2}} \\ &\simeq \left[ (c^\perp(t) \sin \phi_M)^2 + \left\{ c^\perp(t) \left( 1 - \frac{\delta\theta_M^2}{2} \right) \cos \phi_M + c^\parallel(t) \delta\theta_M \right\}^2 \right]^{\frac{1}{2}} \\ &\simeq c^\perp(t) \left[ 1 + 2 \left( \frac{c^\parallel(t)}{c^\perp(t)} \cos \phi_M \right) \delta\theta_M + \left\{ \left( \frac{c^\parallel(t)}{c^\perp(t)} \right)^2 - \cos^2 \phi_M \right\} \delta\theta_M^2 \right]^{\frac{1}{2}} \\ &\simeq c^\perp(t) \left[ 1 + \left( \frac{c^\parallel(t)}{c^\perp(t)} \cos \phi_M \right) \delta\theta_M + \frac{1}{2} \left\{ \left( \frac{c^\parallel(t)}{c^\perp(t)} \right)^2 \sin^2 \phi_M - \cos^2 \phi_M \right\} \delta\theta_M^2 \right]. \end{aligned} \quad (\text{S24})$$

According to the above calculation, the ratio  $c^\perp(t + \delta t)/c^\perp(t)$  deviates more from unity as  $c^\parallel(t)/c^\perp(t)$  is larger, due to the first-order term with respect to  $\delta\theta_M$ . Even if the vortex axis moves so that  $\phi_M = \pm\pi/2$  and the first-order term of  $\delta\theta_M$  vanishes, the second-order term also causes the same tendency to  $c^\perp(t + \delta t)/c^\perp(t)$ . In other words, if the cluster has small radii ( $R_o, R_i$ ) and is extended along the vortex axis, the radial distance changes rapidly due to the motion of the vortex axis. For a large  $\lambda$ , the cluster shape becomes a rotating ball with the aspect ratio close to one, and therefore the correlation decays rapidly.

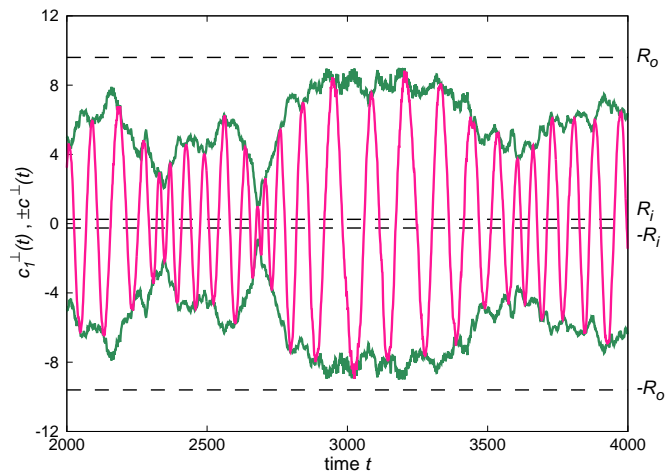

FIG. S8. Time evolution of the radial distance  $c^\perp(t)$  of a certain agent, and  $c_1^\perp(t) = c^\perp(t) \cos \phi(t)$  where  $\phi(t)$  is the azimuthal angle in the projected plane ( $N = 3000, N_u = 3, \lambda = 7.0$ ). The measurement is performed in the same manner as in Fig. 4.

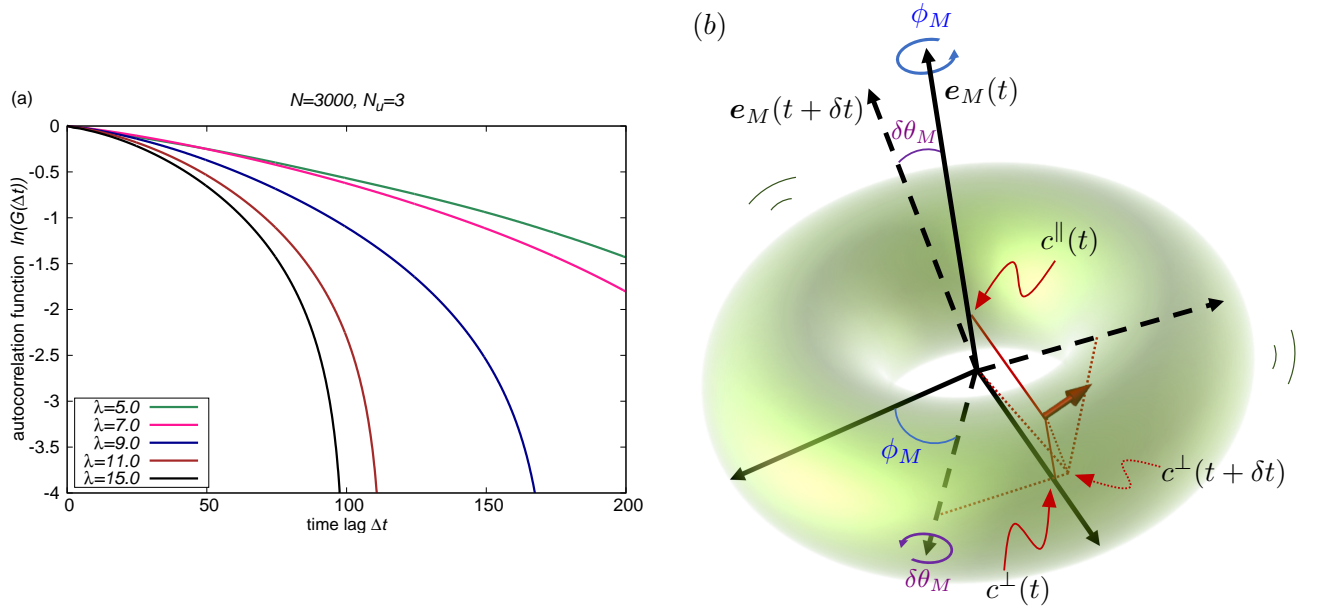

FIG. S9. Figures for understanding the time evolution of the radial distance. (a) Lin-log plots of normalized autocorrelation function  $G(t)$  with  $N = 3000, N_u = 3$ . Green:  $\lambda = 5.0$  (ring). Magenta:  $\lambda = 7.0$  (torus). Blue:  $\lambda = 9.0$  (torus). Brown:  $\lambda = 11.0$  (torus). Black:  $\lambda = 15.0$  (rotating ball). Time-averaging is performed between  $t = 2500$  and  $t = 12500$  with 100000 steps. (b) Schematic picture of the motion of the vortex axis. The green torus represents a torus-shaped cluster, and the red arrow within the green torus is an agent (see the text for details).

## VI. The Size of a Rotating Cluster and Orbital Period

The orbital period of the  $i$ -th agent is obtained as the time interval between the moments at which  $\phi_i(t)$  jumps from  $\pi$  to  $-\pi$  or vice versa. The orbital periods are then averaged over a time interval of duration 500 to calculate

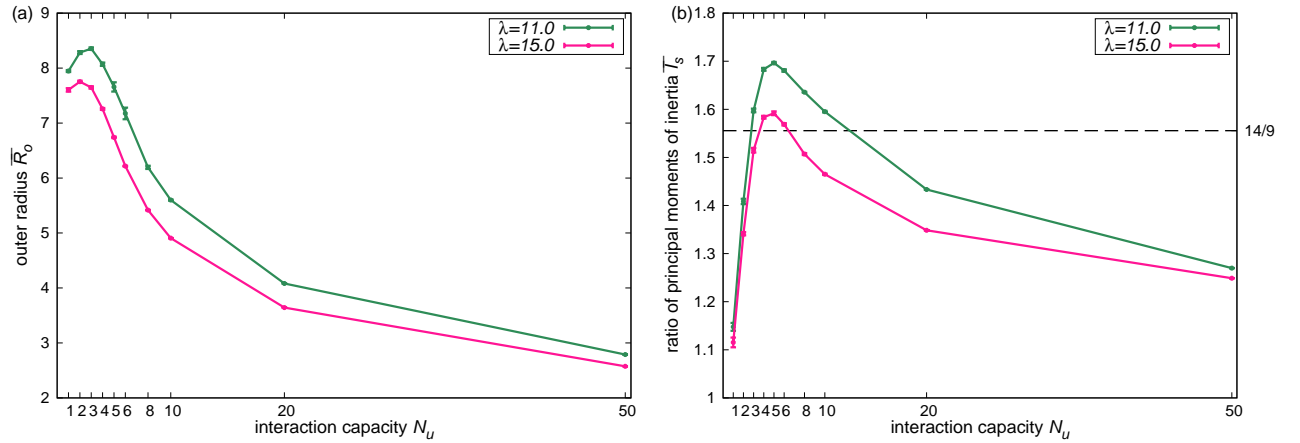

FIG. S10. The shape of vortex-type clusters as a function of the interaction capacity  $N_u$  ( $N = 3000$ ). The solid line represents the arithmetic average of the time-averaged quantities obtained in each of the 10 simulations, and the error bars represent the standard deviation, with the initial condition (ii). The green line shows data for  $\lambda = 11.0$ , and the magenta line for  $\lambda = 15.0$ . (a) The outer radius  $\bar{R}_o$  and (b) the ratio of principal moments of inertia  $\bar{I}_s$  have peaks at a relatively small  $N_u$ , and they continue to decrease from there. In (b), the dashed line shows the criterion of classification between a torus ( $\bar{I}_s > 14/9$ ) and a rotating ball ( $\bar{I}_s \leq 14/9$ ).

the time-averaged orbital period,  $\bar{T}_{i,b}$ . Finally, we average it over the cluster  $\mathcal{C}$  to obtain

$$\bar{T}_b = \frac{1}{|\mathcal{C}|} \sum_{i \in \mathcal{C}} \bar{T}_{i,b}. \quad (\text{S25})$$

The outer radius of the cluster  $\bar{R}_o$  for  $N = 3000$  is plotted as a function of  $N_u$  with the specific values of  $\lambda$  in Fig. S10(a). The cluster diameter is almost comparable to  $r_a$  when  $N_u = 50$ : this is a small cluster in which the cluster size is equal to or smaller than the radius of interaction.  $\bar{R}_o$  is not a monotonously decreasing function of  $N_u$ , and has a peak at some small  $N_u$  depending on  $\lambda$ . This phenomenon is related to the fact that the cluster is very close to a sphere when  $N_u = 1$ , and then at intermediate  $N_u$  it becomes flatter cluster as  $N_u$  is increased from  $N_u = 1$  (see Fig. S10(b)). Note that the difference between the values of  $N_u$  which cause the peak of  $\bar{R}_o$  and  $\bar{T}_s$  comes from the fact that the cluster volume decreases as  $N_u$  increases.

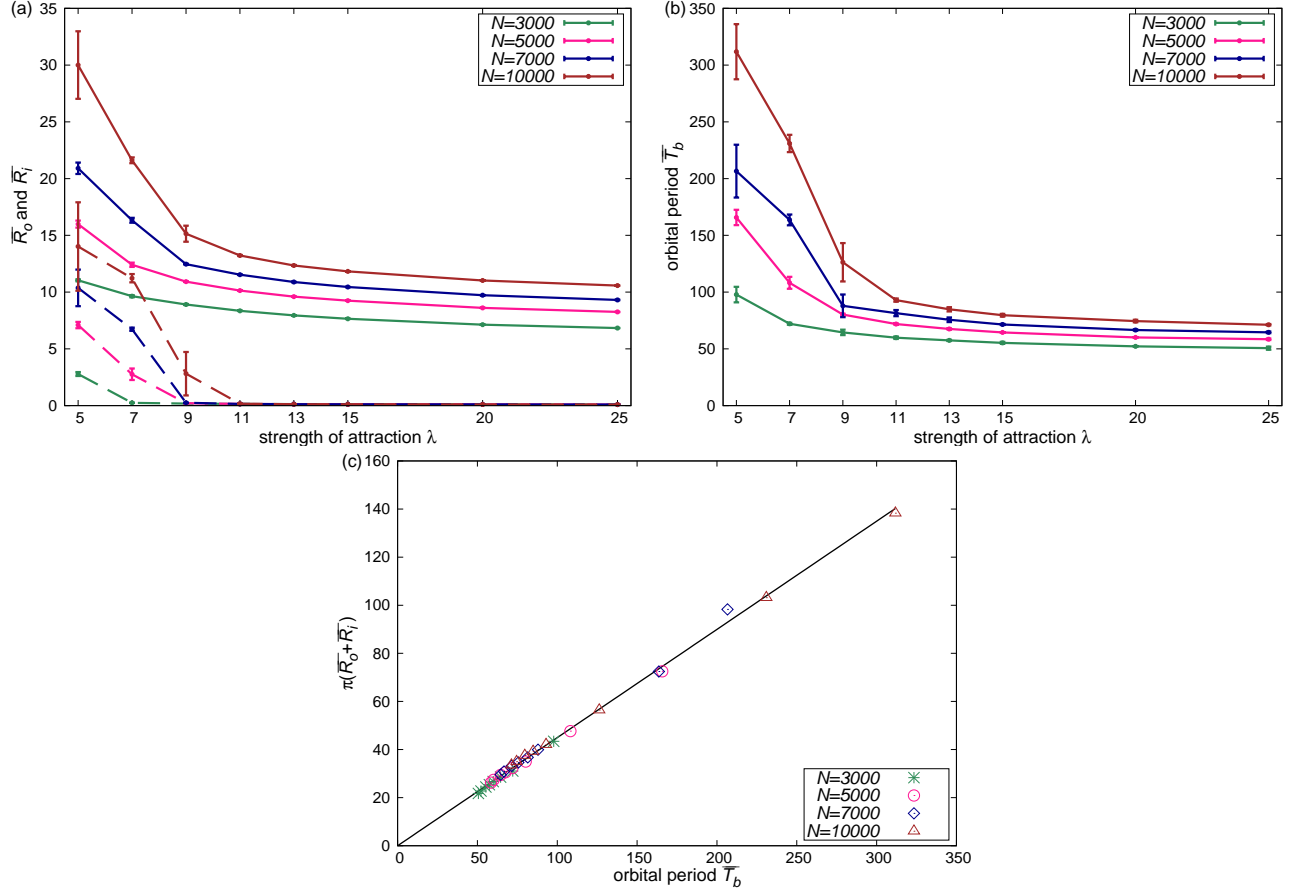

FIG. S11. Dependences of the sizes and rotation period on the number of agents  $N$  for  $N_u = 3$ . The colors of the lines and points correspond to the number of agents as follows. Green:  $N = 3000$ . Magenta:  $N = 5000$ . Blue:  $N = 7000$ . Brown:  $N = 10000$ . Lines and error bars are defined in the same way as Fig. S10. The solid line is  $\bar{R}_o$ , and the dashed line is  $\bar{R}_i$  in (a), and the solid line is  $\bar{T}_b$  in (b). The panel (c) shows the correlation between the average orbit length  $2\pi(\bar{R}_o + \bar{R}_i)/2$  and the period  $\bar{T}_b$ . Fitting by the linear relation  $\pi(\bar{R}_o + \bar{R}_i) = v\bar{T}_b$  gives  $v = 0.45$ , which is represented by the black solid line.

The  $N$ -dependence of the cluster radius and phase diagram for  $N_u = 3$  is shown in Fig. S11(a) and Fig. S12, respectively. As  $\lambda$  increases and the cluster shape transitions from a ring to a rotating ball, both the outer and inner radii ( $\bar{R}_o$ ,  $\bar{R}_i$ ) decrease. Also, as  $N$  increases, rings are formed more easily, and the outer and inner radii increase accordingly.

As for the tangential motion, Fig. S11(b) shows the averaged period  $\bar{T}_b$ . As  $\lambda$  increases, both the period  $\bar{T}_b$  and the cluster radius decrease. The average orbit length of each agent, estimated by  $2\pi(\bar{R}_o + \bar{R}_i)/2$ , is proportional to  $\bar{T}_b$  as shown in Fig. S11(c). The constant of proportionality (averaged tangential velocity within the cluster) is  $v = 0.45$ , which is less than half of  $v_0$ . The fact that this average speed  $v$  is less than half of  $v_0$  will be ascribed to competition

between self-propulsion and repulsive force. In fact, an agent intends to reduce the speed to  $v_0 - v_r = 0$  when it nearly collides with the agent in the front, while it is propelled at the maximum speed  $v_0 = v_r$  to avoid collision with the rear agent. The agent, hence, moves at the speed  $v_0/2$  on average. The speed in the cluster roughly matches with this estimate.

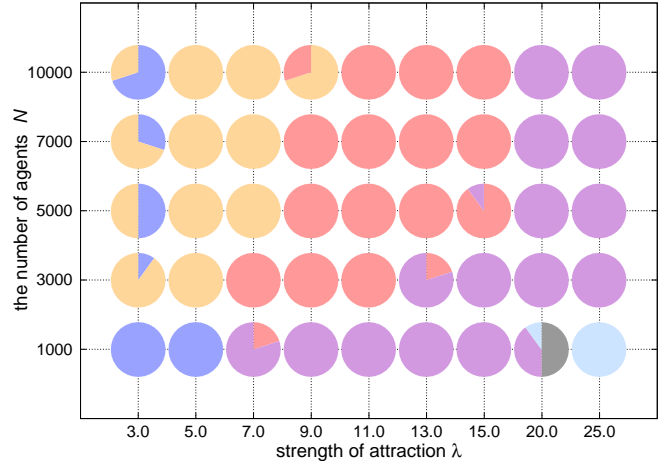

FIG. S12. Phase diagram of the collective motion with  $N_u = 3$ . The pie chart shows the ratio of emergence of each pattern in 10 simulations performed for each parameters  $(\lambda, N)$ . The color corresponds to the pattern in the same way as in Fig. 2.

Fig. S13 provides a supplement to Fig. 3. Fig. S13(a) shows that a rotating cluster is obtained in a wide range of the number of agents  $N$  on the order of 100 to 10000 under fixed parameters ( $N_u = 3, \lambda = 11.0$ ). Fig. S13(b) indicates that, since the inner radius  $\bar{R}_i$  is less than 1 and very small, a rotating cluster is a torus or a rotating ball and there is no large hole in the center. In other words, as the number of agents increases, only the outer radius  $\bar{R}_o$  increases significantly.

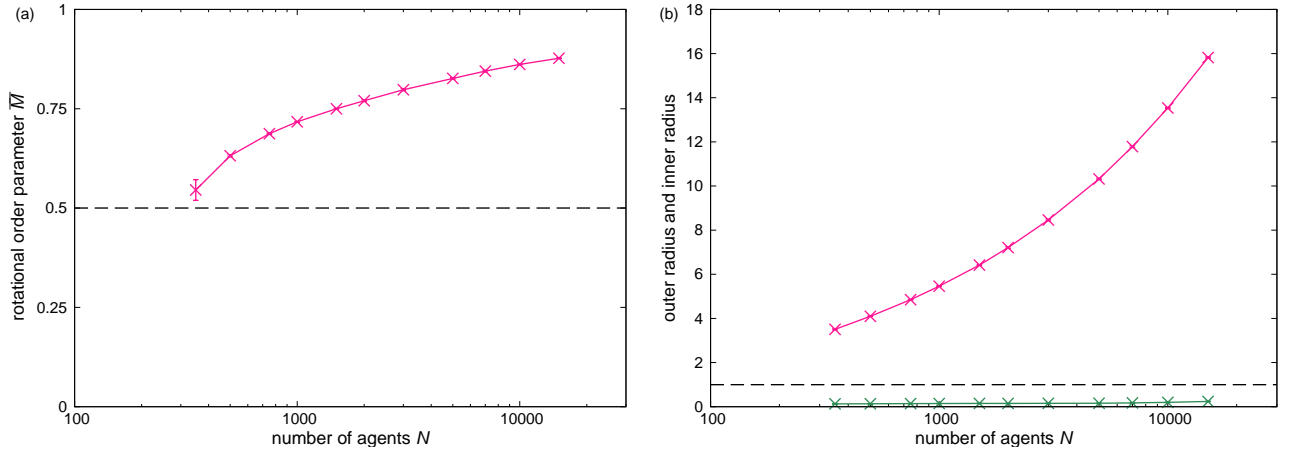

FIG. S13. Dependences of the rotational order parameter, and outer and inner radii on the number of agents  $N$  for  $N_u = 3, \lambda = 11.0$ . We test the cases  $N = 350, 500, 750, 1000, 1500, 2000, 3000, 5000, 7000, 10000$ , and 15000. Lines and error bars are defined in the same way as in Fig. S10. (a) The solid line is the time-averaged rotational order parameter  $\bar{M}$ . The dashed line is  $\bar{M} = 0.5$  which is the criterion of classification between a polarized school and a rotating cluster. (b) The magenta solid line is  $\bar{R}_o$ , and the green solid line is  $\bar{R}_i$ . The dashed line shows the criterion of classification between a ring and other rotating clusters.

## VII. Spatial Distribution

We investigate the spatial distributions of the number density and occupancy ratio  $\eta = |\mathcal{L}|/N_u$  as functions of the radial distance  $c^\perp$  from the axis of rotation of the cluster. We define the density distribution  $\tilde{\rho}(c^\perp, t)$  of the vortex-type cluster as follows.

$$\tilde{\rho}(c^\perp, t) = \sum_{i \in \mathcal{C}} \frac{\delta(c_i^\perp(t) - c^\perp)}{c^\perp}, \quad (\text{S26})$$

where  $c^\perp = |c^\perp|$ , and  $\delta(c_i^\perp(t) - c^\perp)$  is the Dirac delta function. Numerically, we use the bin width  $\Delta c^\perp = 0.01$ , and the  $\delta$ -function is replaced by the number of agents in the interval  $[c^\perp, c^\perp + \Delta c^\perp]$ . Then we calculate the normalized density distribution

$$\rho(c^\perp, t) = \frac{\tilde{\rho}(c^\perp, t)}{\int_0^\infty dc^\perp c^\perp \tilde{\rho}(c^\perp, t)}, \quad (\text{S27})$$

and its time-average  $\bar{\rho}(c^\perp)$ .

As can be seen from Fig. S14(a), the time-averaged and normalized density distribution  $\bar{\rho}(c^\perp)$  has a peak which gets narrower as  $\lambda$  increases. Interestingly, the peak is located at finite radial distances not only for a torus and a ring, but also for a rotating ball. Moreover, this holds even for the case  $N_u = 1$ , where the rotating ball is very close to a sphere (see Fig. S10(b) and Fig. S14(b)). This is explained as follows. In order to sustain the speed  $v_0$ , the agents near the center must change their orientation rapidly, which is difficult due to orientational interaction. Therefore, the agents are repelled from the vortex axis and the density distribution has a dip at the center.

The distribution of the occupancy ratio is

$$\eta(c^\perp, t) = \sum_{i \in \mathcal{C}} \eta_i(t) \delta(c_i^\perp(t) - c^\perp), \quad (\text{S28})$$

where  $\eta_i(t) = |\mathcal{L}_i(t)|/N_u$  is the occupancy ratio. Here, the summation is taken over the time steps when  $\rho(c^\perp, t) > 0$ , because the occupancy ratio has a physical meaning only if there is an agent in the bin.

The distribution of the occupancy ratio  $\eta$  shows the position of the agents that are attracted by others (see Fig. S14(a)). Inside the cluster, the time averaged value of  $\bar{\eta}(c^\perp)$  is almost equal to 1, which means that the agents have mostly orientational and repulsive interactions, and that the interaction radius is smaller than  $r_e$ . Whereas, in the surface regions of the clusters (of width  $\sim r_e$ ),  $\bar{\eta}(c^\perp)$  is smaller than unity, which means that the agents near the surface are attracted by those in the inner part of the cluster. Namely, the majority of the agents repel and reorient each other inside the cluster, and a relatively small number of agents on the surface constantly prevent the cluster from being dispersed by the attraction. Unlike the case where all agents simultaneously have repulsive and attractive interactions, the region where the attractive force acts on agents and the region where the repulsive force acts are spatially separated spontaneously, and this is considered to be essential in formation of a giant rotating cluster.

The distribution of the speed is

$$V(c^\perp, t) = \sum_{i \in \mathcal{C}} |v_i(t)| \delta(c_i^\perp(t) - c^\perp). \quad (\text{S29})$$

The time-averaging is performed only at the time step when  $\rho(c^\perp, t) > 0$  as well as  $\eta(c^\perp, t)$ . The dependence of the speed on the radial position is shown in Fig. S15. We find that the speed is almost constant inside the cluster, and is larger at the surfaces at the outer and inner radii. This is because the agents near the surfaces are attracted by those inside and become faster.

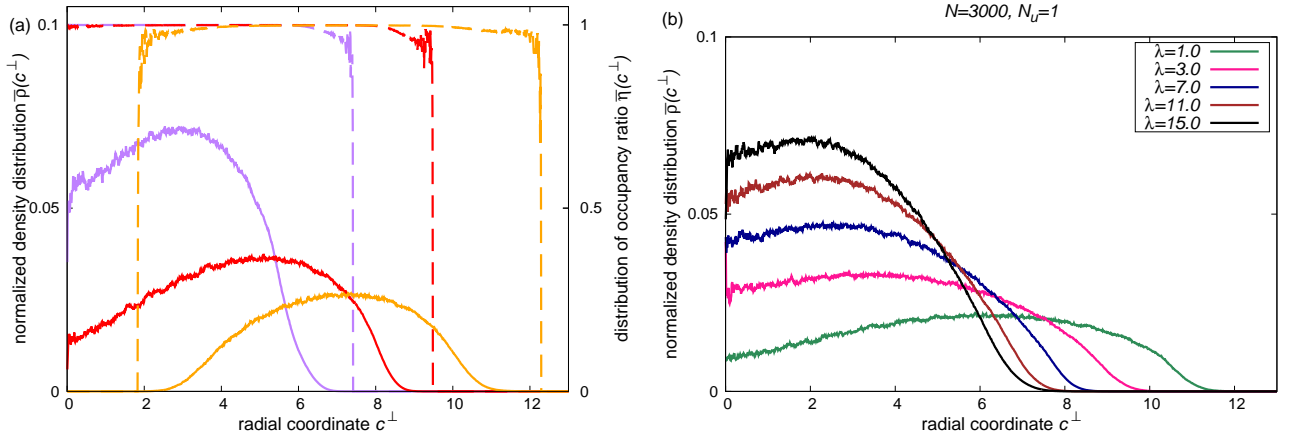

FIG. S14. (a) Structure of a ring and torus and rotating ball for  $N = 3000, N_u = 3$ . Solid lines are normalized density distributions  $\bar{\rho}(c^\perp)$ , and dashed lines are distributions of occupancy ratio  $\bar{\eta}(c^\perp)$ . Both of them are time-averaged. Each line corresponds to the parameters as follows: Orange:  $\lambda = 5.0$  (ring). Red:  $\lambda = 9.0$  (torus). Purple:  $\lambda = 25.0$  (rotating ball). (b) Normalized density distributions  $\bar{\rho}(c^\perp)$  with  $N = 3000, N_u = 1$ . Green:  $\lambda = 1.0$  (torus). Magenta:  $\lambda = 3.0$  (rotating ball). Blue:  $\lambda = 7.0$  (rotating ball). Brown:  $\lambda = 11.0$  (rotating ball). Black:  $\lambda = 15.0$  (rotating ball). They have peaks at finite radial distance.

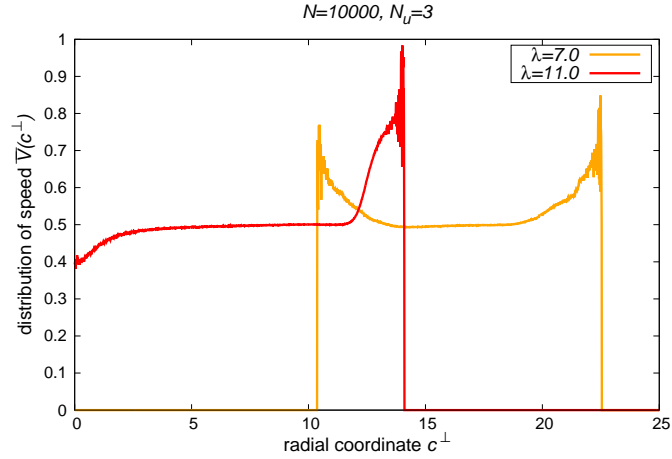

FIG. S15. The distribution of the speed  $\bar{V}(c^\perp)$  for  $N = 10000$ , and  $N_u = 3$ . Orange:  $\lambda = 7.0$  (ring). Red:  $\lambda = 3.0$  (torus). Both clusters increase in the speed on the surfaces. The speed decreases in the center of the torus because of the orientational interaction.

### VIII. Qualitative Explanation for the Shape and the Mechanism of the Patterns

The dependences of the patterns on  $N_u$  and  $\lambda$  in the phase diagram is understood as follows. First of all, we focus on the rotating cluster. Rotating balls are obtained for large  $\lambda$ , because strong attraction tends to minimize the distance between agents. As we decrease  $\lambda$ , the net attraction acting on the surface region is weakened and the cluster is broadened by repulsion, causing the transitions from the ball to a torus (with a small hole in the center) and then to a ring (a large hole). As  $\lambda$  is further decreased, attraction cannot suppress the density fluctuation, and the ring tears off and eventually splits. For a small value of  $N_u$ , the total repulsive force acting on each agent is orientationally random, and some of the agents are repelled along the vortex axis. This explains the transition from a torus to a ball with decrease of  $N_u$ . A rotating ball appears even though  $N_u$  is large, but this does not contradict the above explanation. For large  $N_u$ , strong attraction causes a small cluster and each agent can interact with almost all agents in the cluster (the cluster size  $\lesssim r_a$ ), and hence the net interaction becomes a centripetal force. This explains

formation of compact vortices in previous numerical studies and in the region of large  $N_u$  in our phase diagram, and is completely different from the mechanism that leads to the formation of giant cluster as we find for small  $N_u$ .

Next, the formation of a rotating cluster from an aligned non-rotating cluster, as found in the recovery of a ring from a worm-like cluster (Movie S7 in Ref. [30]), is understood as follows. As shown in Fig. S16, the agents in the front of a cluster are attracted from those following them and change orientation. Then this reorientation propagates to the rear part of the cluster by orientational interaction. Thus the rotational symmetry is spontaneously broken and the cluster starts rotating. Strong attraction (large  $\lambda$ ) enhances change of orientation of the agents in the front,

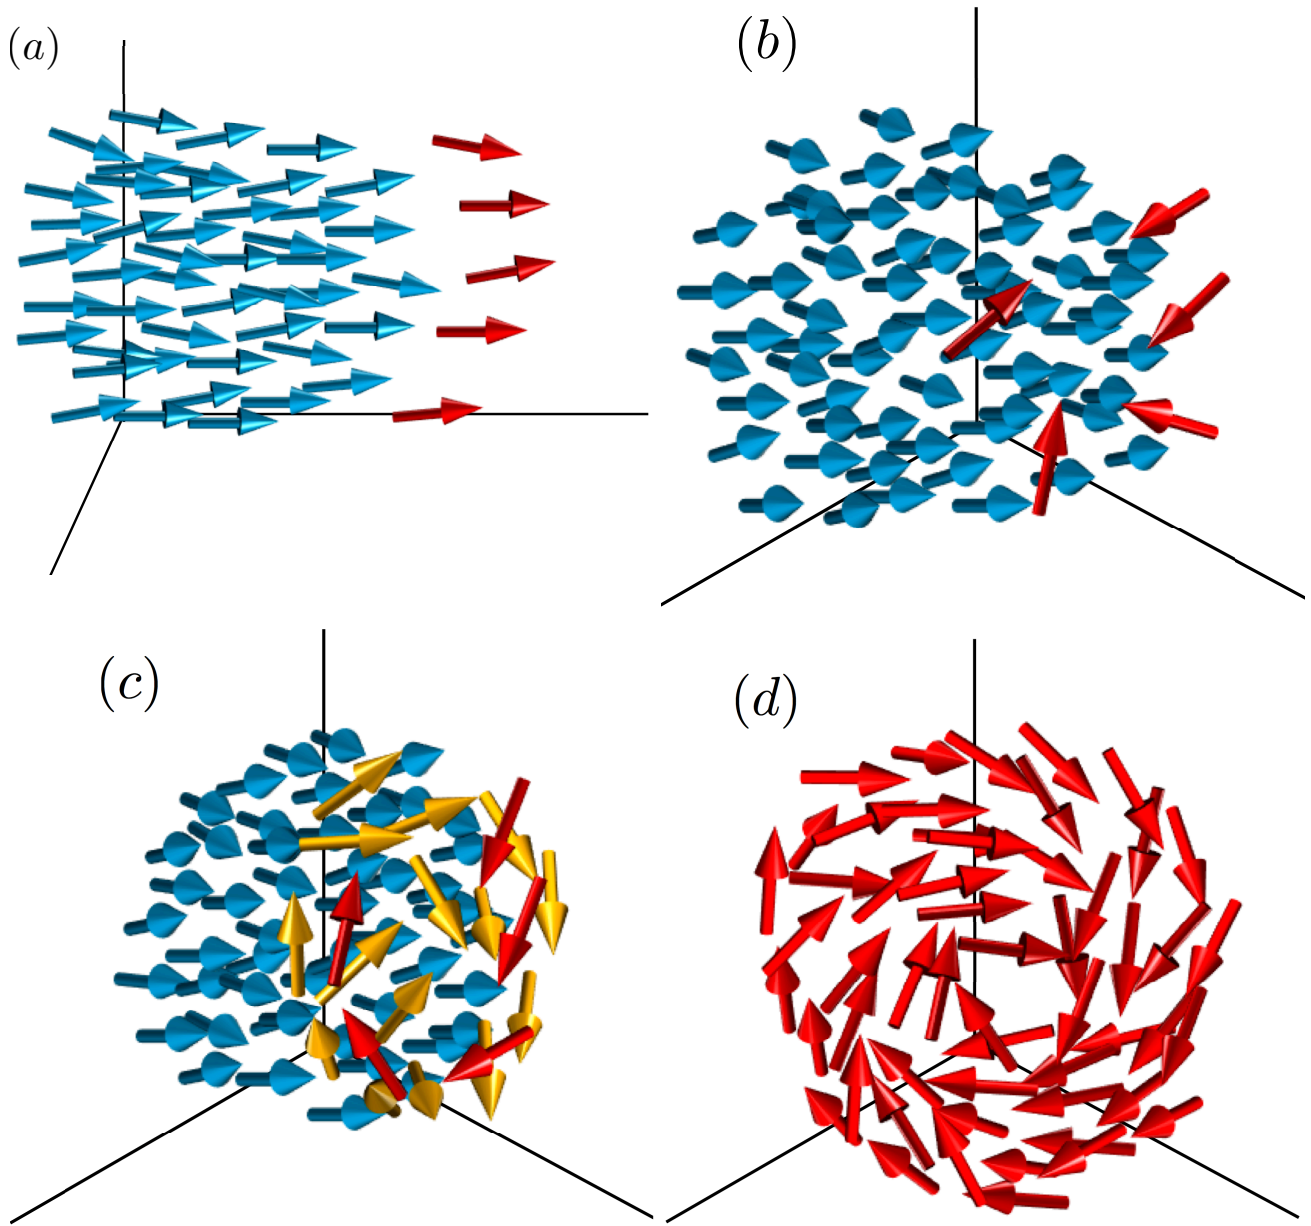

FIG. S16. Schematic picture of the mechanism of formation of a rotating cluster. For simplicity, we consider an aligned cluster in the initial state. An agent is represented by an arrow. The panel (a) is a side view, and (b), (c), and (d) are three-quarter views. (a) The agents in the front (red arrows) that have  $|\mathcal{L}| = N_u$  is pushed out by repulsive force. The number of agents within radius  $r_e$  from these agents becomes less than  $N_u$  ( $|\mathcal{L}| < N_u$ ). (b) Attraction acts on the red arrows, and they attempt to get inside the cluster and change orientation. (c) The agents (yellow arrows) near the surface of the cluster interact with the reoriented agents (red arrows), and gradually align with them by orientation interaction. As the other agents (blue arrows) move forward from behind, they will also align. (d) This step is repeated and finally a rotating cluster is formed.

and a small  $N_u$  makes it possible for the following agents to change its orientation sensitively with a small number of agents in the front. Therefore, vortex-type clusters are frequently obtained in the region of small  $N_u$  and large  $\lambda$  (see Fig. 2). In the case where the agents are randomly oriented in the initial state, local orientational order is formed first in each part of the cluster. The different parts are further aligned by orientational interaction and the whole cluster is almost ordered, and then starts to rotate from the front as described above.

Finally, we explain the relation between the non-rotating cluster and the parameter sets. A polarized school appears frequently at small  $\lambda$  because the agents on the surface of the cluster change velocity only slightly by the attraction and the orientation interaction predominates. When  $N_u$  is large and  $\lambda$  is small, the orientation interaction is averaged between large numbers of agents, and thus the polarized school is easily formed with larger  $\lambda$ . On the other hand, the polarized school also emerges at large  $N_u$  and large  $\lambda$ , because of the smallness of the cluster in which the orientation interaction becomes stronger by the excluded volume effect. An undetermined form appears when the cluster starts to rotate where  $N_u$  is large and the orientation interaction is predominant, but the rotation is not stable due to the intermediate value of  $\lambda$ . A swarm emerges when each agent changes its orientation sensitively with a small number of agents and the agents on the surface of a cluster change its velocity strongly due to a large  $\lambda$ .

- 
- [1] M.R. D’Orsogna, Y.L. Chuang, A.L. Bertozzi, and L.S. Chayes, Phys. Rev. Lett. **96**, 104302 (2006).
  - [2] Z. Cheng, Z. Chen, T. Vicsek, D. Chen, and H.T. Zhang, New J. Phys. **18**, 103005 (2016).
  - [3] N.H.P. Nguyen, E. Jankowski, and S.C. Glotzer, Phys. Rev. E **86**, 011136 (2012).
  - [4] Y.L. Chuang, T. Chou, and M.R. D’Orsogna, Phys. Rev. E **93**, 043112 (2016).
  - [5] N. Shimoyama, K. Sugawara, T. Mizuguchi, Y. Hayakawa, and M. Sano, Phys. Rev. Lett. **76**, 3870 (1996).
  - [6] D. Strömbom, J. Theor. Biol. **283**, 145 (2011).
  - [7] L. Barberis and F. Peruani, Phys. Rev. Lett. **117**, 248001 (2016).
  - [8] D. Strömbom, M. Siljestam, J. Park, and D.J.T. Sumpter, Eur. Phys. J. Spec. Top. **224**, 3311 (2015).
  - [9] A. Costanzo and C.K. Hemelrijk, J. Phys. D: Appl. Phys. **51**, 134004 (2018).
  - [10] A. Costanzo, Europhys. Lett. **125**, 20008 (2019).
  - [11] I.D. Couzin, J. Krause, R. James, G.D. Ruxton, and N.R. Franks, J. Theor. Biol. **218**, 1 (2002).
  - [12] D.S. Calovi, U. Lopez, S. Ngo, C. Sire, H. Chaté, and G. Theraulaz, New J. Phys. **16**, 015026 (2014).
  - [13] A. Filella, F. Nadal, C. Sire, E. Kanso, and C. Eloy, Phys. Rev. Lett. **120**, 198101 (2018).
  - [14] C. M. Breder, Ecology **35**, 361 (1954).
  - [15] We read data from FIG. 1 in Ref. [3].
  - [16] We read data from FIG. 2 in Ref. [13]. ( $r_0$  is the swimmer size.)
  - [17] K. Terayama, H. Hioki, and M. Sakagami, Inter. J. Semantic Comput. **9**, 143 (2015).
  - [18] T. Vicsek, A. Czirók, E. Ben-Jacob, I. Cohen, and O. Shochet, Phys. Rev. Lett. **75**, 1226 (1995).
  - [19] J. Gautrais, F. Ginelli, R. Fournier, S. Blanco, M. Soria, H. Chaté, and G. Theraulaz, PLoS Comput. Biol. **8**, e1002678 (2012).
  - [20] Y. Katz, K. Tunström, C.C. Ioannou, C. Huepe, and I.D. Couzin, Proc. Natl. Acad. Sci. U.S.A. **108**, 18720 (2011).
  - [21] J.E. Herbert-Read, A. Perna, R.P. Mann, T.M. Schaerf, D.J.T. Sumpter, and A.J.W. Ward, Proc. Natl. Acad. Sci. U.S.A. **108**, 18726 (2011).
  - [22] T.Y. Wu, in *Scale Effects in Animal Locomotion*, edited by T.J. Pedley (Academic Press, London/New York, 1977), p. 203.
  - [23] J.J. Videler and C.S. Wardle, Rev. Fish Biol. Fish **1**, 23 (1991).
  - [24] G.V. Lauder and E.D. Tytell, Fish Physiology **23**, 425 (2005).
  - [25] C. Katopodis and R. Gervais, River Res. Applic. **28**, 444 (2012).
  - [26] E.D. Tytell, Proc. R. Soc. Lond. B **271**, 2535 (2004).
  - [27] T.N. Wise, M.A.B. Schwalbe, and E.D. Tytell, J. Exp. Biol. **221**, jeb190892 (2018).
  - [28] P. Domenici and R.W. Blake, J. Exp. Biol. **200**, 1165 (1997).
  - [29] P.W. Webb, J. Exp. Biol. **74**, 211 (1978).
  - [30] For the dynamics, see the supplementary movies at <https://sites.google.com/view/movies-arxiv210605892>.
